# Supplementary material for: In-Hand Manipulation of Unknown Objects with Tactile Sensing for Insertion
Source: arXiv:2210.13403 source file (2023-03-10)
Supplement: Supplementary file 1 [file appendix.tex]

\subsection{Detailed Experiment Results}

\begin{figure}[H]
    \centering
    \includegraphics[width=\linewidth]{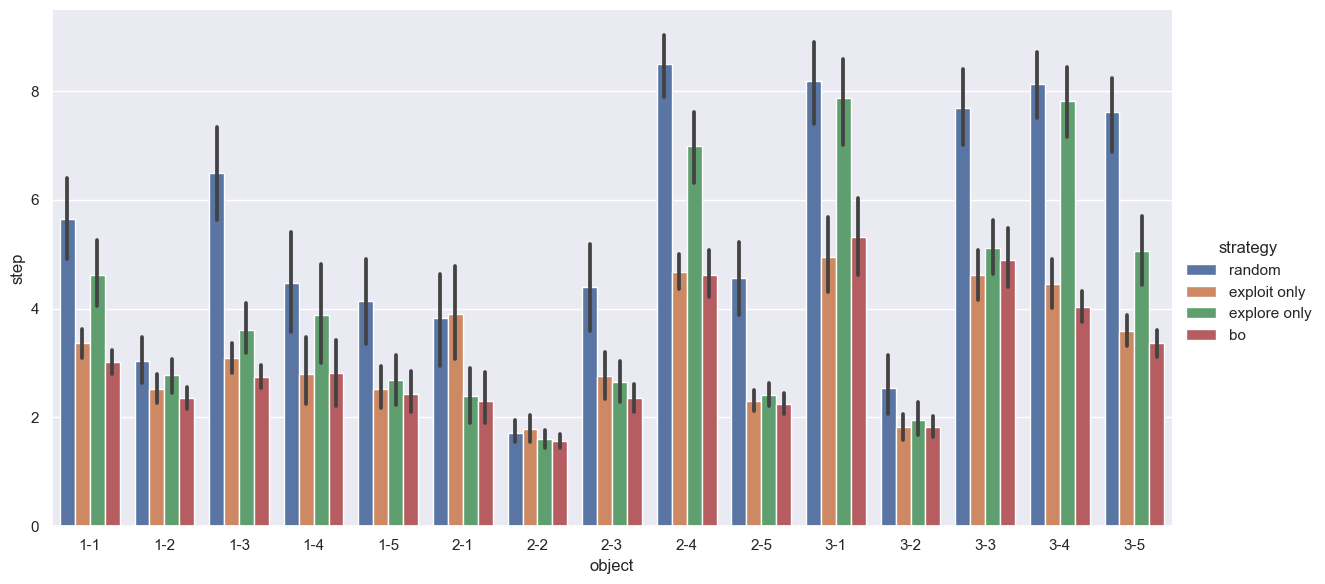}
    \caption{This plot shows the steps to finish the task of different object shapes with PyBullet simulation data. }
    \label{fig:exp:main:step_15shape}
\end{figure}

\begin{figure}[H]
    \centering
    \includegraphics[width=\linewidth]{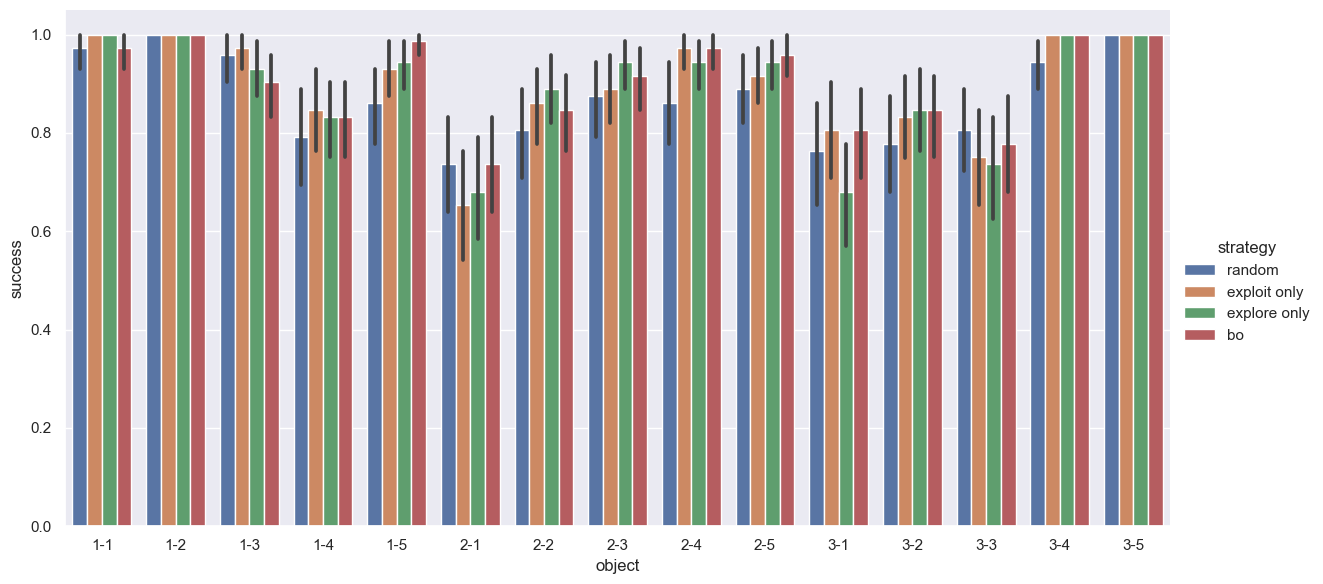}
    \caption{The insertion task success rate over different test objects and strategies. }
    \label{fig:exp:main:success_15shape}
\end{figure}

\subsection{Chaoyi's rewrite of approach section}
First we randomly select a cross section of the object, defined by parameters $\zeta$, $\psi$, and $d$, as shown in Fig. \ref{fig:FullObjParam}. We then rotate the object along this section and collect proprioception and tactile data that we convert into a partial point cloud, as described in Section \ref{SectionShapeEstimation}. Next, we use a GP to build a probabilistic estimate of the global shape of the object from this partial point cloud, as described in Section \ref{GaussianShapeEstimate}.

\begin{figure}[htp]
    \centering
    \includegraphics[width=8cm]{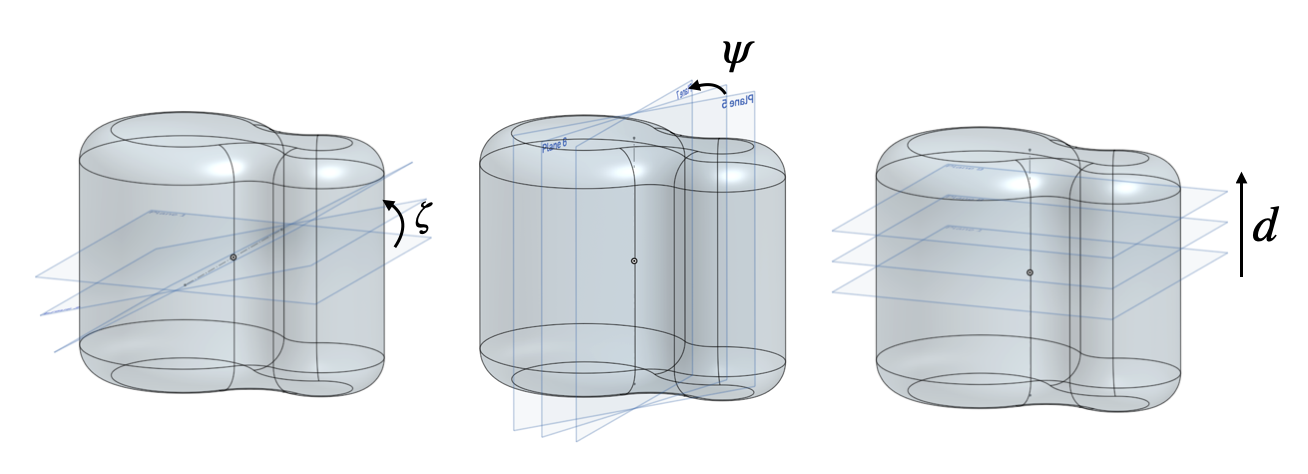}
    \caption{Parameters of the object cross sections.}
    \label{fig:FullObjParam}
\end{figure}

We parameterize the object orientations relative to the target hole with angles $\alpha$, $\beta$, $\gamma$, as shown in \ref{fig:HoleParameterization}. For each orientation, we output a score of how likely the object is to fit into the hole. To do this, we analyze the cross sections of the object along the vertical axis of the hole shown in Fig. \ref{fig:HoleParameterization}. 

\begin{figure}[htp]
    \centering
    \includegraphics[width=8cm]{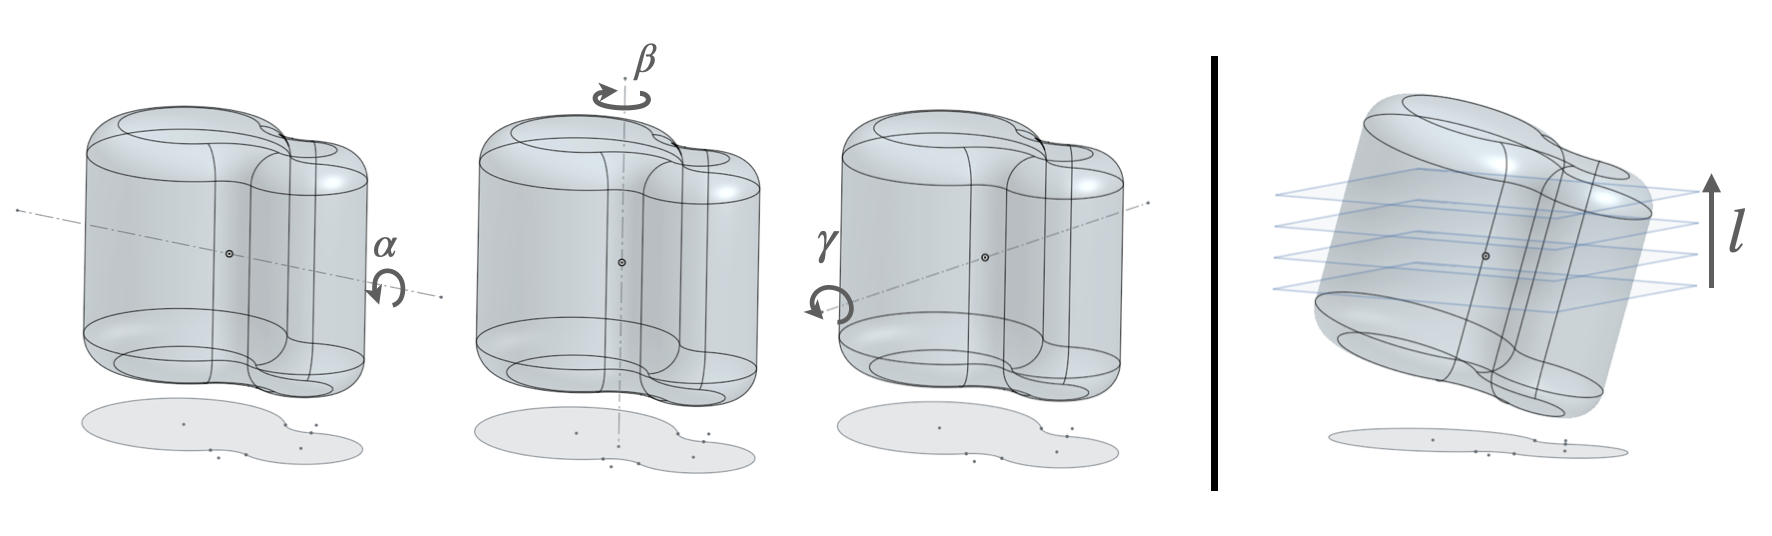}
    \caption{Left: Object orientations relative to the target hole parameterized by angles $\alpha$, $\beta$, $\gamma$. Right: The cross sections along the vertical axis of the hole that need to be analyzed given an orientation of the object. }
    \label{fig:HoleParameterization}
\end{figure}

For calculating the optimal insertion orientation and determining which section to explore next, our pipeline starts by evaluating the margin distribution between the hole and the object in its current orientation.

As the first step, we calculated the probabilistic model of the object in its current orientation. The probabilistic object model is a Gaussian Process in a spherical coordinate system $r(\theta, \phi) \sim \mathcal{N}(\bar{f}, \mathbb{V}[f])$. Considering we need to do projection and getting maximum value over the object model, we first evaluate the Gaussian Process to get the multi-variant Gaussian distribution to represent object shape.  The evaluation points is sampled from different angles in spherical coordinate system by step $\Delta \theta$ and $\Delta \phi$.

\begin{equation}
    \begin{aligned}
        \Theta = & [\mathbf{\theta_0^T}, \mathbf{\theta_1^T}, \cdots ,\mathbf{\theta_{N-1}^T}]^T \in \mathbb{R}^{MN} \\
        \Phi =  & [\mathbf{\phi_0^T}, \mathbf{\phi_1^T}, \cdots ,\mathbf{\phi_{M-1}^T}]^T \in \mathbb{R}^{MN}
    \end{aligned}
\end{equation}

where $\mathbf{\theta_i} = [0, \Delta \theta ,\cdots, (M-1)\Delta \theta]^T \in \mathbb{R}^{M}, \mathbf{\phi_i} = [i\Delta \phi , i\Delta \phi , \cdots , i\Delta \phi]^T \in \mathbb{R}^{N}, M=\frac{2\pi}{\Delta \theta}, N =   \frac{\pi}{\Delta \phi}$. By evaluating Gaussian Process in the given mesh grid angles, we get a joint Gaussian Distribution:

\begin{equation}
    \begin{aligned}
        R_{\text {trans}} = & [\mathbf{{r^t_0}}^T, \mathbf{{r^t_1}}^T, \cdots ,\mathbf{{r^t_{N-1}}}^T]^T \in \mathbb{R}^{MN} \\
        R_{\text {trans}} \sim & \mathcal{N}\{\bar{f}(\Theta, \Phi), \mathbb{V}(f(\Theta, \Phi))\}
    \end{aligned}
\end{equation}

where $\mathbf{r^t_i} = [r^{tr}_{0,i} , r^{tr}_{1,i} , \cdots , r^{tr}_{(M-1),i}]^T \in \mathbb{R}^{M}$. 

In the second step, the object is projected to $x\textit{-}y$ plane to calculate the projection shape. 

\begin{equation}
    \begin{aligned}
        R_{\text {proj}} = & [\mathbf{{r^p_0}}^T, \mathbf{{r^p_1}}^T, \cdots ,\mathbf{{r^p_{N-1}}}^T]^T \in \mathbb{R}^{MN} \\
        R_{\text {proj}} \sim & \mathcal{N}\{\bar{f}(\Theta, \Phi) \odot \cos{\Phi}), \mathbb{V}(f(\Theta, \Phi))\odot \cos{\Phi\Phi^T}\}
    \end{aligned}
\end{equation}

where $\mathbf{r^p_i} = [r^{pr}_{0,i} , r^{pr}_{1,i} , \cdots , r^{pr}_{(M-1),i}]^T \in \mathbb{R}^{M}$. Note that we only need the most protrusive part of the object when calculating the minimum margin to pass a hole. So we calculate the contour distribution by calculating the maximum radius given different angle coordinates. 

\begin{equation}
    \begin{aligned}
        R_{\text{contour}} = & [r^c_0, r^c_1 , \cdots, r^c_{M-1}]^T
    \end{aligned}
\end{equation}

where $r^c_i = \max_{j\in[0,N-1]}{r^{pr}_{i,j}}$. To calculate the distribution of $R_\text{contour}$, we need to calculate the maximum value of a joint Gaussian Distribution \cite{multinormal} \cite{skewgaussian}. By definition of $R_{\text{contour}}$, we have $P(R_{\text{contour}}\le R^c) = P(R_{\text{proj}}<R^{cc})$, where $R^c = [r^c_0, r^c_1, \cdots, r^c_{(M-1)}]\in \mathbb{R}^{M}, R^{cc} = [R^c, R^c, \cdots, R^c] \in \mathbb{R}^{MN}$. 

% \begin{equation}
%     \begin{aligned}
%     F_{R_{\text{contour}}} = \prod_{i=0}^{M-1} \prod_{j=0}^{N-1} & \int_{-\infty}^{r^c_i}{d r^p_{i,j}} f_{R_\text{proj}}(R_\text{proj}) \\
%     \end{aligned}
% \end{equation}

\begin{equation}
    \begin{aligned}
    F_{R_{\text{contour}}} = & \int_{-\infty}^{r^c_0}{d r^p_{0,0} \int_{-\infty}^{r^c_0}} d r^p_{0,1} \cdots \int_{-\infty}^{r^c_0}{d r^p_{0,(N-1)}}  \\
    & \int_{-\infty}^{r^c_1} d r^p_{1,0} \int_{-\infty}^{r^c_1} {dr^p_{1,1}} \cdots \int_{-\infty}^{r^c_1}{dr^p_{1,(N-1)}} \cdots \\
    & \int_{-\infty}^{r^c_{(M-1)}}{dr^p_{(M-1),0}} \int_{-\infty}^{r^c_{(M-1)}}{dr^p_{(M-1),1}} \cdots \\ & \int_{-\infty}^{r^c_{(M-1)}}{dr^{p}_{(M-1),(N-1)}} f_{R_\text{proj}}(R_\text{proj}) \\
    \end{aligned}
\end{equation}

\begin{equation}
    f_{R \text {contour }}=\frac{d F_{R \text {contour }}}{d R}
\end{equation}

At last step, we can calculate the minimum margin distribution when the object passing the hole. By calculating the difference between the hole shape and the object projection contour, we can get the distribution of margin over different angles: $ R_{\text{margin}} = [r^m_0, r^m_1, \cdots,r^m_{M-1}]^T = R_{\text{hole}} - R_{\text{contour}}$. Then, we can calculate the minimum value of the margin distribution and get the minimum margin value when the object passes the hole $r_{\text{margin}} = \min_{i\in[0,M-1]}{r^m_i}$. 

\begin{equation}
    \begin{aligned}
        F_{r_{\text{margin}}}(r) = & 1 - P (r_1 \le r, r_2 \le r, \cdots, r_{M-1} \le r )\\
        = & 1 - 
        \int_{r_{\text{margin}}}^{+ \infty}{d r_{m,0}}
        \int_{r_{\text{margin}}}^{+ \infty}{d r_{m,1}}
        \cdots \\ 
        & \int_{r_{\text{margin}}}^{+ \infty}{d r_{m, M-1}}
        F_{R_{\text{margin}}}(r^m_0, r^m_1, \cdots,r^m_{M-1})
    \end{aligned}
\end{equation}

\begin{equation}
    f_{r_{\text{margin}}} = \frac{d F_{r \text { margin }}}{d r}
\end{equation}

In practice, we calculate the mean and variance of margin size by Monte Carlo algorithm. After calculating the transformed jointed object shape distribution $ R_{\text {trans}} \sim \mathcal{N}\{\bar{f}(\Theta, \Phi) \odot \cos{\Phi}), \mathbb{V}(f(\Theta, \Phi))\odot \cos{\Phi\Phi^T}\} $, we sample $K$ data to a series of object shapes $R_{\text{trans},1}, R_{\text{trans},2}, \cdots, R_{\text{trans},K}$. Then we can calculate the projected object shape $R_{\text{proj},i}=R_{\text{trans},i} \odot \cos{\Phi}$. Similarly, we can calculate the contour shape through $ R_{\text{contour}, i} = [r^c_0, r^c_1 , \cdots, r^c_{M-1}]^T, \mathbf{r^p_i} = [r^{pr}_{0,i} , r^{pr}_{1,i} , \cdots , r^{pr}_{(M-1),i}]^T \in \mathbb{R}^{M}$. At last step, we can calculate the margin size $R_{\text{margin}, i} = [r^m_0, r^m_1, \cdots,r^m_{M-1}]^T = R_{\text{hole}} - R_{\text{contour}, i},  r_{\text{margin}, i} = \min_{i\in[0,M-1]}{r^m_i}$.

\subsection{Original more detailed version of approach section}
Note that for a given $\theta$ angle on the $x\textit{-}y$ plane, the most protruding part of the object section will limit its ability to fit through the hole. Therefore, we are interested in taking the maximum of $R^{\text{proj}}_{m,n}$ over all $\phi_n$ for a given $\theta_m$. Hence, we define the  planar contour distribution as the distribution of  the random variable $R_m^{\text{cntr}}:=\max_{n}{R^{\text{proj}}_{m,n}}$.
To compute the distribution of $R_m^{\text{cntr}}$, we need to calculate the maximum value of a joint Gaussian distribution as in \cite{multinormal, skewgaussian}: 
\begin{align} \label{int1}
    F_{R_m^{\text{cntr}}}(r_m^{\text{cntr}}) &= \prod_{n} P(R_{m,n}^{\text{proj}} \leq r_m^{\text{cntr}} )= \prod_{n}\! \int_{-\infty}^{r_m^{\text{cntr}}} \!\! dF_{R_{m, n}^{\text{proj}}} %\\
    % &= \prod_{n} \int_{-\infty}^{\bar{r_{m}^{\text{cntr}}} f_{R_m^{\text{cntr}} dr
\end{align}

% From this cdf, we can obtain the pdf $f_{r_m^{\text{cntr}}$ as $\frac{dF_{r_m^{\text{cntr}}}{dr}$.
Thus, we have a distribution describing the object contour at angle $\theta_m$ in the plane of the hole (the $x\textit{-}y$ plane). 

\begin{figure}[t]
    \vspace{7px}
    \centering
    \includegraphics[width=7cm]{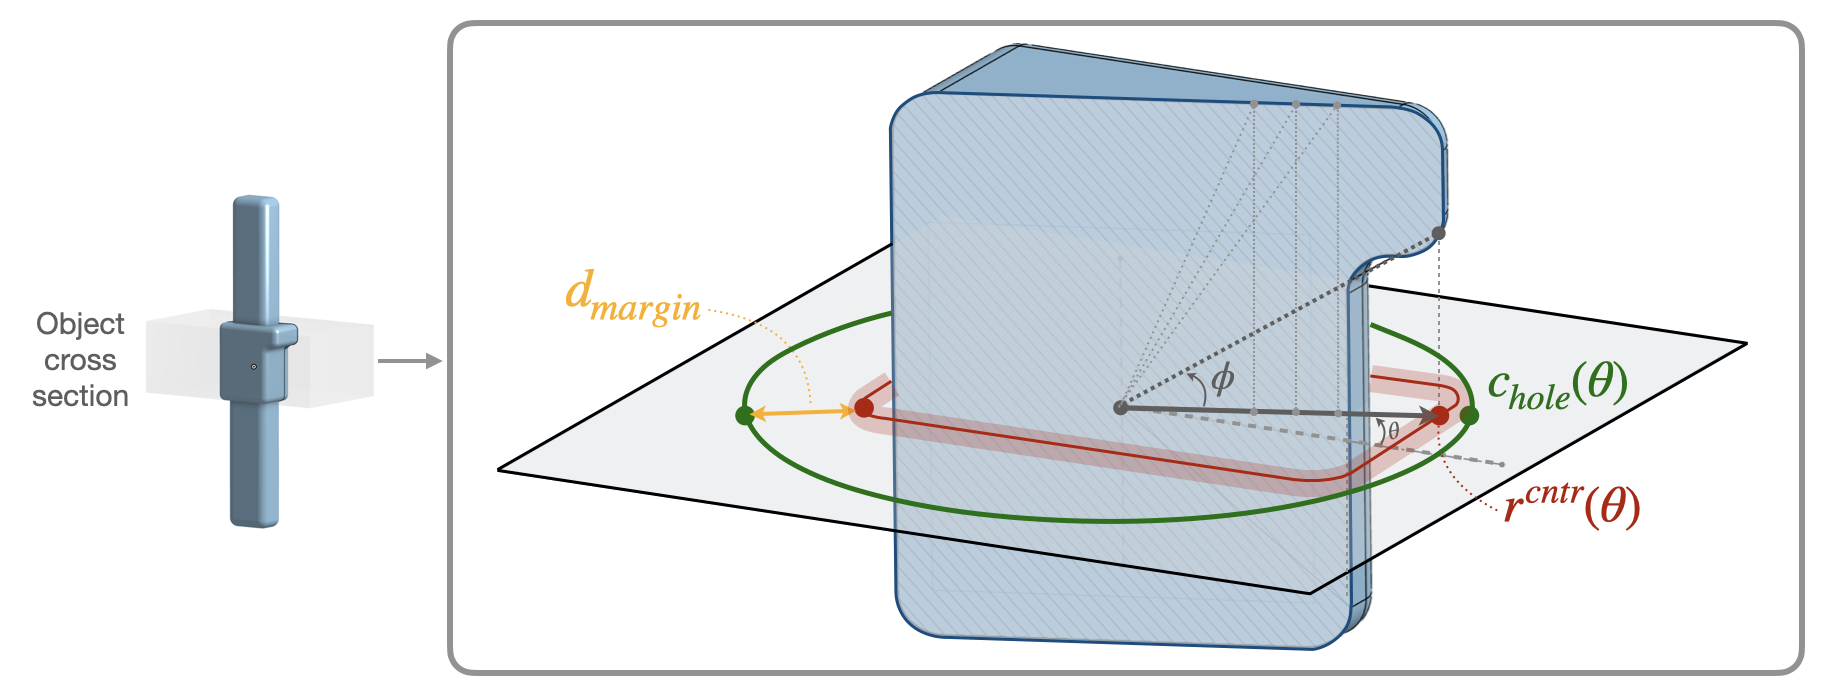}
    \caption{For a given cross section of the object, this figure shows how the points on the object are projected onto a plane. We compare this projected contour to the contour of the hole to evaluate the fit of the object.}
    \label{fig:bo_explanation}
    \vspace{-5px}
\end{figure}

Our goal is to produce a score for the current object orientation and section. Conceptually, this score should correspond to how likely this object section is to collide with the hole, which is dominated by the part of the object that is most likely to overlap with the edge of the hole (or is closest to the edge of the hole). Thus, for the current orientation, we want to compute the distribution that describes the maximum overlap (equivalently, the minimum margin between the object and the hole). We obtain this distribution $D_m$ at each $\theta_m$ as: $ D_m = c^{\text{hole}}_m - R^{\text{cntr}}_m$, where $c^{\text{hole}}_m$ is a known scalar describing the hole radius at angle $\theta_m$.
% \begin{equation}
%     d_i = r^{\text{hole}}_m - r^c_m
% \end{equation}

Finally, we can calculate $\min_m{D_m}$ over all possible $\theta_m$ to obtain the score distribution $S$ for the current orientation and section; again as in \cite{multinormal, skewgaussian}:
\begin{align} \label{int2}
    F_{S}(s) &= \prod_{m} P(s \leq D_m )= 1 - \prod_{m} \int_{s}^{\infty} dF_{D_m} %\\
    % &= \prod_{n} \int_{-\infty}^{\bar{r_{m}^{cont}}} f_{r_m^{cont}} dr
\end{align}
